# Supplementary material for: Learning Physics-guided Face Relighting under Directional Light
Source: arXiv:1906.03355 source file (2020-04-19)
Supplement: Supplementary file 1 [file sec_supplementary.tex]

\section{Supplementary Material}
%\balance

% \section{Relighting with Environment Maps}
% As explained in %Sec.~5.3 
% \cref{sec:extensions} 
% in the main paper, we can relight an input image w.r.t.~a given environment map through sampling. In addition to 
% %Fig.~6 in the main paper,
% \cref{fig:experiments:envMap},~\cref{fig:experiment:envmap1,fig:experiment:envmap2} show relighting results for $5$ different environment maps, ranging from cold to warm color temperatures.

\subsection{Dataset Details}\label{sec:appendix:datasetDetails}
In order to balance the demographics of the captured data, we split the $21$ subjects into a training, validation and test set according to~\cref{tab:supp:datasetDetails}, to achieve a meaningful distribution of salient characteristics in all of the subsets.

\begin{table}[h]
\caption{{\bf Dataset Details.} Considerations of salient characteristics to balance training, validation and test set.
}
\label{tab:supp:datasetDetails}
\centering
% \small
% \begin{tabular}{ccccccc}
% \toprule
%            & female   & dark skin   & bald    & beard    & glasses \\
% \midrule
% training   & $2$      & $3$         & $1$     & $7$      & $4$ \\
% validation & $1$      & $1$         & $1$     & $1$      & $1$ \\
% test       & $1$      & $1$         & $0$     & $1$      & $1$ \\
% \midrule                
% total      & $4$      & $5$         & $2$     & $9$      & $6$ \\
% ratio      & $19.0\%$ & $23.8\%$    & $9.5\%$ & $42.9\%$ & $28.6\%$ \\
% \bottomrule
% \end{tabular}
\begin{tabular}{ccccc}
\toprule
           & female   & dark skin   & glasses \\
\midrule
training   & $2$      & $3$         & $4$ \\
validation & $1$      & $1$         & $1$ \\
test       & $1$      & $1$         & $1$ \\
\midrule                
total      & $4$      & $5$         & $6$ \\
ratio      & $19.0\%$ & $23.8\%$    & $28.6\%$ \\
\bottomrule
\end{tabular}
\end{table}

\subsection{Dynamic Input Lighting}
We illustrate the consistency and robustness of our approach by relighting multiple source light configurations to the same target lighting in~\cref{fig:experiment:inputLightDependence1,fig:experiment:inputLightDependence2}. Our examples cover a wide spectrum of source illuminations, including strong and challenging directional lights originating on the side of the face. The extreme cases on the far left and right, in particular, require the removal of strong shadows. The noise in these low light areas is high, and visual cues are weak, which makes consistent relighting challenging.
% Please also refer to the video\youtube, where we show results in a dynamic environment with moving lights.

\subsection{Extended Results}
An extended comparison to related work can be found in~\cref{fig:experiment:comparison1,fig:experiment:comparison2}. More results on relighting with an environment map are available in~\cref{fig:experiment:envmap1,fig:experiment:envmap2}. Additional results of relighting under a moving target illumination can be found in the supplemental video\youtube.

%%%%%%%%%%%%%%%%%%%%%%%%%%%%%%%%%%%%%%%%%%%%%%%%%%%%%%%%%%%%%%%%%%%%%%%%%%%%%%%%
\def\imgsize{1.0\linewidth}
\begin{figure*}[t]
\centering
\includegraphics[width=\imgsize]{figures/supplementary/performanceBasedOnInput/150918-400004-0000.jpg}\\
\includegraphics[width=\imgsize]{figures/supplementary/performanceBasedOnInput/150911-400004-0000.jpg}\\
\includegraphics[width=\imgsize]{figures/supplementary/performanceBasedOnInput/150917-400004-0000.jpg}\\
\includegraphics[width=\imgsize]{figures/supplementary/performanceBasedOnInput/150903-400004-0000.jpg}\\
\caption{{\bf Dynamic Input Lighting.} In each row, we show a different facial expression that we relight from different input light configurations (columns; see small inset) to the same target light configuration. All results are based on our ``full guidance'' model and have been converted from linear to sRGB.
}
\label{fig:experiment:inputLightDependence1}
\end{figure*}

\begin{figure*}[t]
\centering
\includegraphics[width=\imgsize]{figures/supplementary/performanceBasedOnInput/150900-400004-0500.jpg}\\
\includegraphics[width=\imgsize]{figures/supplementary/performanceBasedOnInput/150911-400004-0500.jpg}\\
\includegraphics[width=\imgsize]{figures/supplementary/performanceBasedOnInput/150901-400004-0500.jpg}\\
\includegraphics[width=\imgsize]{figures/supplementary/performanceBasedOnInput/150908-400004-0500.jpg}\\
\caption{{\bf Dynamic Input Lighting.} In each row, we show a different facial expression that we relight from different input light configurations (columns; see small inset) to the same target light configuration. All results are based on our ``full guidance'' model and have been converted from linear to sRGB.
}
\label{fig:experiment:inputLightDependence2}
\end{figure*}

%%%%%%%%%%%%%%%%%%%%%%%%%%%%%%%%%%%%%%%%%%%%%%%%%%%%%%%%%%%%%%%

\def\tabsize{20.3mm}
\def\tabwhite{20.9mm}
% \newcolumntype{C}[1]{>{\centering\let\newline\\\arraybackslash\hspace{0pt}}m{#1}}
\def\imgsize{1.0\linewidth}

\begin{figure*}[t]
\centering
\includegraphics[width=\imgsize]{figures/supplementary/comparisons/150903-400004-0004-0009.jpg}\\
\includegraphics[width=\imgsize]{figures/supplementary/comparisons/150908-400004-0010-0025.jpg}\\
\includegraphics[width=\imgsize]{figures/supplementary/comparisons/150913-400004-0017-0001.jpg}\\
\includegraphics[width=\imgsize]{figures/supplementary/comparisons/150915-400004-0026-0006.jpg}\\
\includegraphics[width=\imgsize]{figures/supplementary/comparisons/150906-400004-0018-0017.jpg}\\

\begin{tabular}{C{\tabwhite}C{\tabsize}C{\tabsize}C{\tabsize}C{\tabsize}C{\tabsize}C{\tabwhite}}
(a) input image & (b) SfSNet {\small(pretrained)} & (c) SfSNet (retrained) & (d) no guidance & (e) partial guidance & (f) full guidance & (g) ground truth
\end{tabular}
\caption{{\bf Extended Baseline Comparisons.} We compare relighting ({\bf a})~the input image with ({\bf b}/{\bf c})~pretrained and retrained variants of SfSNet~\cite{sengupta2018sfsnet}, ({\bf d})~our model with no guidance as an extension of pix2pix~\cite{isola2017pix2pix}, ({\bf e})~our model with partial guidance on the normals, and ({\bf f})~our model with full guidance. In ({\bf g}), we show the ground truth capture of the given target illumination. All results have been converted from linear to sRGB.
}
\label{fig:experiment:comparison1}
\end{figure*}

\begin{figure*}[t]
\centering
\includegraphics[width=\imgsize]{figures/supplementary/comparisons/152601-400004-0025-0019.jpg}\\
\includegraphics[width=\imgsize]{figures/supplementary/comparisons/152604-400004-0028-0026.jpg}\\
\includegraphics[width=\imgsize]{figures/supplementary/comparisons/151709-400004-0010-0004.jpg}\\
\includegraphics[width=\imgsize]{figures/supplementary/comparisons/151711-400004-0008-0028.jpg}\\
\includegraphics[width=\imgsize]{figures/supplementary/comparisons/151712-400004-0018-0017.jpg}\\

\begin{tabular}{C{\tabwhite}C{\tabsize}C{\tabsize}C{\tabsize}C{\tabsize}C{\tabsize}C{\tabwhite}}
(a) input image & (b) SfSNet {\small(pretrained)} & (c) SfSNet (retrained) & (d) no guidance & (e) partial guidance & (f) full guidance & (g) ground truth
\end{tabular}
\caption{{\bf Extended Baseline Comparisons.}
We compare relighting ({\bf a})~the input image with ({\bf b}/{\bf c})~pretrained and retrained variants of SfSNet~\cite{sengupta2018sfsnet}, ({\bf d})~our model with no guidance as an extension of pix2pix~\cite{isola2017pix2pix}, ({\bf e})~our model with partial guidance on the normals, and ({\bf f})~our model with full guidance. In ({\bf g}), we show the ground truth capture of the given target illumination. All results have been converted from linear to sRGB.
}
\label{fig:experiment:comparison2}
\end{figure*}

%%%%%%%%%%%%%%%%%%%%%%%%%%%%%%%%%%%%%%%%%%%%%%%%%%%%%%%%%%%%%%%%%%%%%%%%%%%%%%%%
\def\envOne{uffizi-0000}
\def\envTwo{esplanade-0000}
\def\envThree{grace-0127}
\def\envFour{grace-0000}
\def\envFive{fire-0127}

\def\imgsize{0.157\linewidth}
\begin{figure*}[t]
\centering
\def\subject{150901}
\includegraphics[width=\imgsize]{figures/supplementary/envmaps/\subject-400004-0009_real_A_sRGB.jpg}
\hspace{0.025\linewidth}
\includegraphics[width=\imgsize]{figures/supplementary/envmaps/\subject-400004-0009-\envOne_envMap_sRGB.jpg}
\includegraphics[width=\imgsize]{figures/supplementary/envmaps/\subject-400004-0009-\envTwo_envMap_sRGB.jpg}
\includegraphics[width=\imgsize]{figures/supplementary/envmaps/\subject-400004-0009-\envThree_envMap_sRGB.jpg}
\includegraphics[width=\imgsize]{figures/supplementary/envmaps/\subject-400004-0009-\envFour_envMap_sRGB.jpg}
\includegraphics[width=\imgsize]{figures/supplementary/envmaps/\subject-400004-0009-\envFive_envMap_sRGB.jpg}
\def\subject{150903}
\includegraphics[width=\imgsize]{figures/supplementary/envmaps/\subject-400004-0009_real_A_sRGB.jpg}
\hspace{0.025\linewidth}
\includegraphics[width=\imgsize]{figures/supplementary/envmaps/\subject-400004-0009-\envOne_envMap_sRGB.jpg}
\includegraphics[width=\imgsize]{figures/supplementary/envmaps/\subject-400004-0009-\envTwo_envMap_sRGB.jpg}
\includegraphics[width=\imgsize]{figures/supplementary/envmaps/\subject-400004-0009-\envThree_envMap_sRGB.jpg}
\includegraphics[width=\imgsize]{figures/supplementary/envmaps/\subject-400004-0009-\envFour_envMap_sRGB.jpg}
\includegraphics[width=\imgsize]{figures/supplementary/envmaps/\subject-400004-0009-\envFive_envMap_sRGB.jpg}
\def\subject{151705}
\includegraphics[width=\imgsize]{figures/supplementary/envmaps/\subject-400004-0009_real_A_sRGB.jpg}
\hspace{0.025\linewidth}
\includegraphics[width=\imgsize]{figures/supplementary/envmaps/\subject-400004-0009-\envOne_envMap_sRGB.jpg}
\includegraphics[width=\imgsize]{figures/supplementary/envmaps/\subject-400004-0009-\envTwo_envMap_sRGB.jpg}
\includegraphics[width=\imgsize]{figures/supplementary/envmaps/\subject-400004-0009-\envThree_envMap_sRGB.jpg}
\includegraphics[width=\imgsize]{figures/supplementary/envmaps/\subject-400004-0009-\envFour_envMap_sRGB.jpg}
\includegraphics[width=\imgsize]{figures/supplementary/envmaps/\subject-400004-0009-\envFive_envMap_sRGB.jpg}
\def\subject{152600}
\includegraphics[width=\imgsize]{figures/supplementary/envmaps/\subject-400004-0009_real_A_sRGB.jpg}
\hspace{0.025\linewidth}
\includegraphics[width=\imgsize]{figures/supplementary/envmaps/\subject-400004-0009-\envOne_envMap_sRGB.jpg}
\includegraphics[width=\imgsize]{figures/supplementary/envmaps/\subject-400004-0009-\envTwo_envMap_sRGB.jpg}
\includegraphics[width=\imgsize]{figures/supplementary/envmaps/\subject-400004-0009-\envThree_envMap_sRGB.jpg}
\includegraphics[width=\imgsize]{figures/supplementary/envmaps/\subject-400004-0009-\envFour_envMap_sRGB.jpg}
\includegraphics[width=\imgsize]{figures/supplementary/envmaps/\subject-400004-0009-\envFive_envMap_sRGB.jpg}
% \includegraphics[width=\imgsize]{figures/supplementary/envmaps/\subject-400004-0009-\envSix_envMap_sRGB.jpg}
% \def\subject{152604}
% \includegraphics[width=\imgsize]{figures/supplementary/envmaps/\subject-400004-0009_real_A_sRGB.jpg}
% \hspace{0.025\linewidth}
% \includegraphics[width=\imgsize]{figures/supplementary/envmaps/\subject-400004-0009-\envOne_envMap_sRGB.jpg}
% \includegraphics[width=\imgsize]{figures/supplementary/envmaps/\subject-400004-0009-\envTwo_envMap_sRGB.jpg}
% \includegraphics[width=\imgsize]{figures/supplementary/envmaps/\subject-400004-0009-\envThree_envMap_sRGB.jpg}
% \includegraphics[width=\imgsize]{figures/supplementary/envmaps/\subject-400004-0009-\envFour_envMap_sRGB.jpg}
% \includegraphics[width=\imgsize]{figures/supplementary/envmaps/\subject-400004-0009-\envFive_envMap_sRGB.jpg}
% % \includegraphics[width=\imgsize]{figures/supplementary/envmaps/\subject-400004-0009-\envSix_envMap_sRGB.jpg}

\caption{{\bf Relighting with Environment Maps.} We relight the input (first column) w.r.t. $5$ different environment maps (small insets), ordered from cold (second column) to warm (sixth column) dominating color temperatures. All results have been converted from linear to sRGB.
}
\label{fig:experiment:envmap1}
\end{figure*}

% available sequences to choose from:
%'150900',
%'150901',
%'150902',
%'150903',
%'150905',
%'150906',
%'150907',
%'150908',
%'150909',
%'150910',
%'150917',
%'150918',

%'152503',  % glasses

%'152600',
%'152604',

%'151600',  % glasses
%'151603',  % glasses

%'151705',
%'151711',
%'151712',
%'151715',
%'151716',

\begin{figure*}[t]
\centering
\def\subject{150905}
\includegraphics[width=\imgsize]{figures/supplementary/envmaps/\subject-400004-0009_real_A_sRGB.jpg}
\hspace{0.025\linewidth}
\includegraphics[width=\imgsize]{figures/supplementary/envmaps/\subject-400004-0009-\envOne_envMap_sRGB.jpg}
\includegraphics[width=\imgsize]{figures/supplementary/envmaps/\subject-400004-0009-\envTwo_envMap_sRGB.jpg}
\includegraphics[width=\imgsize]{figures/supplementary/envmaps/\subject-400004-0009-\envThree_envMap_sRGB.jpg}
\includegraphics[width=\imgsize]{figures/supplementary/envmaps/\subject-400004-0009-\envFour_envMap_sRGB.jpg}
\includegraphics[width=\imgsize]{figures/supplementary/envmaps/\subject-400004-0009-\envFive_envMap_sRGB.jpg}
\def\subject{151711}
\includegraphics[width=\imgsize]{figures/supplementary/envmaps/\subject-400004-0009_real_A_sRGB.jpg}
\hspace{0.025\linewidth}
\includegraphics[width=\imgsize]{figures/supplementary/envmaps/\subject-400004-0009-\envOne_envMap_sRGB.jpg}
\includegraphics[width=\imgsize]{figures/supplementary/envmaps/\subject-400004-0009-\envTwo_envMap_sRGB.jpg}
\includegraphics[width=\imgsize]{figures/supplementary/envmaps/\subject-400004-0009-\envThree_envMap_sRGB.jpg}
\includegraphics[width=\imgsize]{figures/supplementary/envmaps/\subject-400004-0009-\envFour_envMap_sRGB.jpg}
\includegraphics[width=\imgsize]{figures/supplementary/envmaps/\subject-400004-0009-\envFive_envMap_sRGB.jpg}
\def\subject{151600}
\includegraphics[width=\imgsize]{figures/supplementary/envmaps/\subject-400004-0009_real_A_sRGB.jpg}
\hspace{0.025\linewidth}
\includegraphics[width=\imgsize]{figures/supplementary/envmaps/\subject-400004-0009-\envOne_envMap_sRGB.jpg}
\includegraphics[width=\imgsize]{figures/supplementary/envmaps/\subject-400004-0009-\envTwo_envMap_sRGB.jpg}
\includegraphics[width=\imgsize]{figures/supplementary/envmaps/\subject-400004-0009-\envThree_envMap_sRGB.jpg}
\includegraphics[width=\imgsize]{figures/supplementary/envmaps/\subject-400004-0009-\envFour_envMap_sRGB.jpg}
\includegraphics[width=\imgsize]{figures/supplementary/envmaps/\subject-400004-0009-\envFive_envMap_sRGB.jpg}
\def\subject{152503}
\includegraphics[width=\imgsize]{figures/supplementary/envmaps/\subject-400004-0009_real_A_sRGB.jpg}
\hspace{0.025\linewidth}
\includegraphics[width=\imgsize]{figures/supplementary/envmaps/\subject-400004-0009-\envOne_envMap_sRGB.jpg}
\includegraphics[width=\imgsize]{figures/supplementary/envmaps/\subject-400004-0009-\envTwo_envMap_sRGB.jpg}
\includegraphics[width=\imgsize]{figures/supplementary/envmaps/\subject-400004-0009-\envThree_envMap_sRGB.jpg}
\includegraphics[width=\imgsize]{figures/supplementary/envmaps/\subject-400004-0009-\envFour_envMap_sRGB.jpg}
\includegraphics[width=\imgsize]{figures/supplementary/envmaps/\subject-400004-0009-\envFive_envMap_sRGB.jpg}

\caption{{\bf Relighting with Environment Maps.} We show the same type of visualization as in \cref{fig:experiment:envmap1} but focus on more challenging scenarios, such as expressions affecting the face topology and glasses. All results have been converted from linear to sRGB.
}
\label{fig:experiment:envmap2}
\end{figure*}
